# Supplementary material for: Semi-dual Regularized Optimal Transport
Source: arXiv:1811.05527 source file (2018-11-13)
Supplement: Supplementary file 1 [file appendix.tex]

% !TEX root = ../SIGEST-SemiDual.tex

%SEC A
%\input sections/sec-appendix
\section{Legendre transform with respect to two histograms}\label{sub:two}

Theorem~\ref{thm-legendre-transf} can be extended to study the Legendre transform of $W_\ga(\p,\q)$ with respect to both arguments $(\p,\q)$ instead of only $\p$. Indeed, expression~\eqref{eq-wassdist-dual} shows that $(\p,\q) \mapsto W_\ga(\p,\q)$ is a convex function (as a maximum of linear forms), so that one can define $\foralls (g,h) \in \RR^n \times \RR^n$,
$$	
W^*_\ga(g,h) = \umax{\p,\q \in \Sigma_n} \dotp{g}{\p} + \dotp{h}{\q} - W(\p,\q).
$$

The following proposition adapts  to this \pagebreak setting.

%prop A.1
\begin{proposition}\label{eq-obj-bothvar}
	The function $W^*_\ga$ is $C^\infty$ at $(g,h) \in \RR^n \times \RR^n$ and, writing $K=e^{-M/\ga}$, $\alpha=e^{g/\ga}, \beta=e^{h/\ga}$ and $\Kcal_{\alpha\beta} = \diag(\alpha)K \beta$, we have that
\begin{gather*}% \label{eq-obj-bothvar}
\begin{split}
  		W^*_\ga(g,h) &= -\gamma \log \alpha^TK\beta,\\%\label{eq-grad-bothvar} 
		\nabla W^*_\ga(g,h) &= \frac{1}{\alpha^T K \beta}\begin{bmatrix}\Kcal_{\alpha,\beta} \\ \Kcal_{\beta,\alpha}\end{bmatrix},\\%\label{eq-hessian-bothvar} 
\nabla^2 W_\ga^*(g) &= \frac{1}{\ga\alpha^T K \beta} \begin{bmatrix} A_\gamma(g,h) & B_\gamma(g,h) \\ B_\gamma(h,g ) & A_\gamma(h,g )\end{bmatrix},				
\end{split}
\\
	\qwhereq					
	\begin{cases}
		A_\gamma(g,h) =  \diag(\Kcal_{\alpha\beta})- \frac{1}{\alpha^T K \beta}\Kcal_{\alpha\beta}\Kcal_{\alpha\beta}^T,\\
		B_\gamma(g,h) = \diag(\beta)\K \diag(\alpha)-\frac{1}{\alpha^T K \beta}\Kcal_{\beta\alpha}\Kcal^T_{\alpha\beta}.
	\end{cases}
\end{gather*}
	Moreover, the gradient function $(g,h)\mapsto\nabla W^*_\ga(g,h)$ is $2/\gamma$ Lipschitz.	
\end{proposition}	
\begin{proof}
One has that $W^*_\ga(g,h)$ can be written
\begin{align*}
	 &\umax{p,q\in\Si_n} \dotp{g}{p} + \dotp{h}{q} - \umax{u,v} \dotp{u}{p} + \dotp{v}{q} - \beta_{\ga,M}(u,v)  \\
			 &\quad= \umax{p,q}  -\umax{u,v} \dotp{u+g}{p}  + \dotp{v+h}{q} - \beta_{\ga,M}(u,v) \\
			 &\quad= \umax{p,q}  -\umax{u',v'} \dotp{u'}{p} + \dotp{v'}{q} - \beta_{\ga,M}(u'+g,v'+h) \\
%			 &= \umax{p,q}  -\umax{u',v'} \dotp{u'}{p} + \dotp{v'}{q} - \beta_{\ga,M-g\ones^T - \ones h^T}(u',v') \\
			 &\quad= \umax{p,q}  -W_{M+g\ones^T + \ones h^T}(\p,\q) \\
			 &\quad= \umax{p,q}  - \! \umin{X \in U(\p,\q)} \dotp{X}{M-g\ones^T - \ones h^T} - \ga E(X) \\			 
			 &\quad= - \umin{X\in\Sigma_{n^2}} \dotp{X}{M-g\ones^T - \ones h^T} - \ga E(X).
\end{align*}
One verifies that the last equation is equivalent to a classic maximal entropy problem which can be solved uniquely with a Gibbs distribution equal to $X^\star$ given below,
%\begin{equation}\label{eq:xgh} 
	$$X^\star = \frac{\diag(\alpha) K \diag(\beta)}{\alpha^T K \beta}.$$%\end{equation}
Substituting this expression in the formula above for $W^*_\ga(g,h)$ yields that
$$
W^*_\ga(g,h) = -\gamma \log \alpha^TK\beta.
$$
Since the gradients with respect to $g$ and $h$ of $W^*_\ga(g,h)$ are $X^\star \ones$ and $X^{\star T}\ones$, respectively, this results in the expression provided above. The Hessian follows from that result, and the Lipschitz continuity of the gradient can be obtained by showing that the Hessian's trace can be upper-bounded by $2/\ga$ by noticing that the trace of both $A_\ga(g,h)$ and $A_\ga(h,g)$ is upper-bounded by $\alpha^TK\beta$.\qquad\end{proof}
